# Supplementary material for: Dynamic Deterministic Constant-Approximate Distance Oracles with $n^{\epsilon}$ Worst-Case Update Time
Source: arXiv:2402.18541 source file (2024-04-10)
Supplement: Supplementary file 1 [file A-appendix.tex]

\appendix

\section{Correctness of \Cref{algo:LocalFlow}}
\label{sect:CorrectnessLocalFlow}

\begin{lemma}
At the beginning of the algorithm and the end of each phase, we have $\lambda \leq d_{w}^{(h)}(s,t)$.
\end{lemma}
\begin{proof}
We will prove it by induction. Initially, $\lambda\leq d_{w}^{(h)}(s,t)$ holds by our initialization of $\lambda$ and $w$. Let $\lambda_{i}$ and $w_{i}$ denote $\lambda$ and function $w$ at the end of each phase $i$. For an inductive step $i$, assume for contradiction that, at the end of phase $i$, there is an $h$-length path $P$ has $w_{i}$-weight less then $\lambda_{i} = (1+\epsilon_{0})\lambda_{i-1}$. Then in every iteration of this phase, the path blocker will saturate at least one edge on $P$. Since there are $\Theta(h\log_{1+\epsilon_{0}}(n)/\epsilon_{0})$ iterations in phase $i$, by averaging, there exists an edge $e\in P$ saturated by $\hat{f}$ in at least $\Theta(\log_{1+\epsilon_{0}}(n)/\epsilon_{0})$ iterations. This means $w_{i}(e)\geq (1+\epsilon_{0})^{\Theta(\log_{1+\epsilon_{0}}(n)/\epsilon_{0})}/m^{\zeta}\geq n^{2}$ (by choosing the constant inside the $\Theta$ to be big enough)\thatchaphol{I added this}, a contradiction.\thatchaphol{this is too fast.} 
\end{proof}
